# Supplementary material for: Ideology Detection for Twitter Users with Heterogeneous Types of Links
Source: arXiv:1612.08207 source file (2016-12-24)
Supplement: Supplementary file 1 [file Appendix.tex]

%Appendix A
\appendix
\section{Deduction of Equation 1}
Recall that the cumulative distribution function of the stochastic disturbance is 
$$ F(x) = e^{-e^{-x}} $$
and the probability density function is given by 
$$ f(x) = \frac{dF(x)}{dx} = e^{-x} e^{-e^{-x}} $$
We have 
\begin{equation} \label{equ:ded}
	\begin{aligned}
		p(u_i \to v_j) = &~ P(U_i(\bm{\psi}_j) > U_i(\bm{\zeta}_j)) \\
		= &~ P(\nu_{ij} - \eta_{ij} < u_i(\bm{\psi_j}) - u_i(\bm{\zeta_j})) \\ 
		= &~ P(\nu_{ij} < -||\bm{p}_i-\bm{\psi}_j||^2 + ||\bm{p}_i-\bm{\zeta}_j||^2 + \eta_{ij}) \\
		= &~ P(\nu_{ij} < \bm{p}_i \cdot 2(\bm{\psi}_j - \bm{\zeta}_j) + (||\bm{\zeta_j}||^2 - ||\bm{\psi_j}||^2) + \eta_{ij}) \\
		= &~ P(\nu_{ij} < \bm{p}_i \cdot \bm{q}_j + b_j + \eta_{ij}) \\		
		= &~ \int_{-\infty}^{\infty} P(\nu_{ij} < \bm{p}_i \cdot \bm{q}_j + b_j + \eta_{ij} | \eta_{ij}) 
		 f(\eta_{ij}) d\eta_{ij} \\	
		= &~ \int_{-\infty}^{\infty} F(\bm{p}_i \cdot \bm{q}_j + b_j + \eta_{ij}) f(\eta_{ij}) d\eta_{ij} \\
		= &~ \int_{-\infty}^{\infty} e^{-e^{-(\bm{p}_i \cdot \bm{q}_j + b_j + \eta_{ij})}} 
		 e^{-\eta_{ij}} e^{-e^{-\eta_{ij}}} d\eta_{ij} \\
		= &~ \int_{-\infty}^{\infty} e^{-e^{-\eta_{ij}} \cdot ( 1 + e^{-(\bm{p}_i \cdot \bm{q}_j + b_j)} ) }
		 e^{-\eta_{ij}} d\eta_{ij} \\
	\end{aligned}
\end{equation}

Consider $G(x) = e^{-c \cdot e^{-x}}$. We have 
$$ \frac{d G(x)}{d x} = G(x) \cdot c \cdot e^{-x} $$
Therefore
\begin{equation}
	\begin{aligned}
		 & \int_{-\infty}^{\infty} G(x) e^{-x} dx \\
		= & \frac{1}{c} \int_{-\infty}^{\infty} \frac{d G(x)}{d x} dx \\
		= & \frac{1}{c} (G(\infty) - G(-\infty)) \\ 
		= & \frac{1}{c}
	\end{aligned}
\end{equation}
Replacing $1 + e^{-(\bm{p}_i \cdot \bm{q}_j + b_j)}$ with $c$ in Equation \ref{equ:ded} we have 
\begin{equation}
	p(u_i \to v_j) = \frac{1}{c} = \sigma(\bm{p}_i \cdot \bm{q}_j + b_j)
\end{equation}
